# Supplementary material for: The Submodular Santa Claus Problem in the Restricted Assignment Case
Source: arXiv:2011.06939 source file (2020-11-13)
Supplement: Supplementary file 1 [file appendix_main.tex]

When considering $\alpha$-relaxed perfect matchings
in regular hypergraphs with sufficiently large hyperedges, we can assume that $\ell =300.000\log^{3}(n)$ at a constant loss:

If $\ell$ is smaller than $300.000\log^{3}(n)$, then we simply duplicate all hyperedges an appropriate number of times.
If $\ell$ is larger, we select for each player $300.000\log^{3}(n)$ configurations uniformly at random from his configurations. The expected number of times a resource appears in a configuration with this process is at most $300.000\log^{3}(n)$. Hence, the probability that a resource appears more than $600.000\log^{3}(n)$ times is at most $\exp \left(- 1/3 \cdot 100.000\log^{3}(n)\right)\leq 1/n^{10}$ by a standard Chernoff bound (see Proposition~\ref{cor:chernoff}). Hence with high probability this event does not happen for any resource.
We now have that each player has $300.000\log^{3}(n)$ configurations and each resource does not appear in more than $600.000\log^{3}(n)$ configurations.
Taking for each configuration $C$ only $\lfloor |C| / 2 \rfloor$ resources we can reduce the
latter bound to $300.000\log^3(n)$ as well:
The previous argument gives a half-integral matching of resources to configurations satisfying
the mentioned guarantee. Then by integrality
of the bipartite matching polytope there
is also an integral one.
